# Supplementary material for: Toward a Realistic Benchmark for Out-of-Distribution Detection
Source: arXiv:2404.10474 source file (2024-04-16)
Supplement: Supplementary file 1 [file supplementary.tex]

\appendixpageoff
\appendixtitleoff

\begin{appendices}
\onecolumn
\begin{center}
  \textbf{\large \appendixtocname}
\end{center}
\section{}
\begin{algorithm}
\caption{Training of the OOD Detector $g$}\label{alg:oodl_ocsvm_training}
\begin{algorithmic}
\label{app:supp1}
\Require training dataset features, $\mathcal{X}_{tf}$, validation dataset features $\mathcal{V}_f$

\State $ss \gets StandardScaler()$

\For{\texttt{data batch} $b \in \mathcal{X}_{tf}$}
    \State ss.partial\_fit(b)
\EndFor

\State $\gamma \gets 1/\text{\#features of }\mathcal{X}_{tf}$
\State $best\_score \gets 0$

\For{$\nu \in \{0.5, 0.1, 0.01\}$}
    \For{$kernel \in \{RBFSampler, Nystroem\}$}
        \For{$average \in \{True, False\}$}
            \State $svm \gets SGDOneClassSVM(\nu,average)$
            \State $ker \gets kernel(\gamma)$
            
            \For{\texttt{data batch} $b \in \mathcal{X}_{tf}$}
                \State $x \gets ss.transform(b)$
                \If{$ker$ not fit}
                    \State $ker.fit(x)$
                \EndIf
                \State $x \gets ker.transform(x)$
                \State $svm.partial\_fit(x)$
            \EndFor
            \State $clf \gets make\_pipeline(ker, svm)$
            \State $auc \gets AUROC(ss, clf, \mathcal{V}_f)$
            \If{$auc > best\_score$}
                \State $best\_score \gets auc$
                \State $best\_clf \gets clf$
            \EndIf
        \EndFor
    \EndFor
\EndFor
\State $\textbf{return } make\_pipeline(ss, best\_clf)$
\end{algorithmic}
\end{algorithm}

\begin{algorithm}
\caption{OODL Training}\label{alg:oodl_training}
\begin{algorithmic}
\Require training dataset features, $\mathcal{X}_{tf}$, validation dataset features $\mathcal{V}_f$

\State $candidate\_layers \gets $\{2, 5.0, 5.1, 10.0, 10.1, 15.0, 15.1, 22.0, 22.1, 27.0, 27.1, 34.0, 34.1, 39.0, 39.1, 46.0, 46.1\}

\State $oodl\_score \gets 0$

\For{$l \in candidate\_layers$}
    \State $ft \gets extract\_features\_of\_layer(\mathcal{X}_{tf}, l)$
    \State $fv \gets extract\_features\_of\_layer(\mathcal{V}_{f}, l)$
    \State $d \gets train\_ood\_detector(ft, fv)$ \Comment{see Algorithm~\ref{alg:oodl_ocsvm_training}}
    \State $auc \gets AUROC(d, fv)$
    \If{$auc > oodl\_score$}
        \State $oodl\_score \gets auc$
        \State $oodl \gets l$
    \EndIf
\EndFor

\State $\textbf{return } oodl, oodl\_score$
\end{algorithmic}
\end{algorithm}

\begin{algorithm}[h]
\caption{Prediction similarity computation}\label{alg:prediction_similarity}
\begin{algorithmic}
\Require ground truth class $gt\_label$, predicted class $pred\_label$

\State $gt\_synsets \gets get\_synsets\_for\_class(gt\_label)$

\State $pred\_synsets \gets get\_synsets\_for\_class(pred\_label)$

\State $max\_sim \gets 0$

\For{$s1 \in gt\_synsets$}
    \For{$s2 \in pred\_synsets$}
        \State $sim \gets \frac{Wu\_Palmer\_similarity(s1, s2) + path\_similarity(s1, s2)}{2}$
        \If{$sim > max\_sim$}
            \State $max\_sim \gets sim$
        \EndIf
    \EndFor
\EndFor
\State $\textbf{return } max\_sim$
\end{algorithmic}

\end{algorithm}

% \section{Figures}
% \label{app:supp2}

\begin{figure}
    \centering
    \includegraphics[width=0.7\textwidth]{images/filtered_t1_graph.pdf}
    \caption[Pruned version of the original graph.]{Pruned version of the original graph, with no Intra-Dataset, obviously correct nor noisy edges. Width and darkness of a link are proportional to the weight. Each node's position is determined by applying the ForceAtlas2 algorithm for graph visualization~\cite{jacomy2014forceatlas2}.}
    \label{fig:filtered_t1_graph}
\end{figure}

\end{appendices}
